# Supplementary material for: Kinetic Effects in Dynamic Wetting
Source: arXiv:1702.01916 ancillary file (2017-02-07)
Supplement: Supplementary file 1 [file kineticwetting_supplementary3.pdf]

# Kinetic Effects in Dynamic Wetting (Supplementary Material)

James E. Sprittles*
*Mathematics Institute, University of Warwick, CV4 7AL*
(Dated: February 6, 2017)

The Supplementary Material contains technical details that are complementary to the (self-complete) Letter including (a) a full mathematical problem formulation which contains additional details of the lubrication model developed, (b) benchmark simulations establishing the limits of applicability of the lubrication approach and (c) results for confined menisci.

## PROBLEM FORMULATION

Consider the two-dimensional flow generated by the steady motion of a smooth chemically-homogeneous solid surface which is driven through a liquid-gas free surface in a direction aligned with gravity at a constant speed $U$. Here, a dimensional formulation will be presented but a non-dimensional scheme can be found in [1]. The dynamics are first formulated for the full two-dimensional setup, with hydrodynamics used in both bulk phases, which is used to validate our Lubrication Formulation (into which the Boltzmann equation can be incorporated).

*Bulk flow.* The flow of a fluid with constant density $\rho$ and viscosity $\mu$ is described by the steady incompressible Navier-Stokes equations

$$\nabla \cdot \mathbf{u} = 0, \qquad \rho(\mathbf{u}\cdot\nabla)\mathbf{u} = \nabla\cdot\mathbf{P} + \rho\mathbf{g},$$

where $\mathbf{P} = -p\mathbf{I} + \mu\left[\nabla\mathbf{u} + (\nabla\mathbf{u})^T\right]$ is the stress tensor, $\mathbf{u}$ is the velocity, $p$ is the local pressure, $\mathbf{I}$ is the metric tensor, and $\mathbf{g}$ is the acceleration due to gravity. These equations apply in both the liquid and gas phases, and when required subscripts $l$ and $g$ will be used to refer to their respective components.

*Solid boundary.* The solid moves with velocity $\mathbf{U}$ and has outward normal $\mathbf{n}$. The conditions of impermeability and slip on the liquid-solid and liquid-gas boundaries can be written as

$$\mathbf{u}\cdot\mathbf{n} = 0, \qquad l_{slip}\,\mu^{-1}\,\mathbf{n}\cdot\mathbf{P}\cdot(\mathbf{I}-\mathbf{nn}) = \mathbf{u}_{\parallel} - \mathbf{U}_{\parallel},$$

where $l_{slip}$ is the slip length which (a) on the liquid-solid interface is fixed at $l_{slip} = 10$ nm [2] and (b) on the gas-solid interface (i) is $l_{slip} = 10$ nm for the *no-slip model* but (ii) depends on the mean free path $l_{slip} = \alpha\,\ell$ for the *slip model*, where Knudsen layers are accounted for. The components of a vector parallel to a surface are $\mathbf{a}_{\parallel} = \mathbf{a}\cdot(\mathbf{I}-\mathbf{nn})$.

*Free surface.* The dynamics of the liquid and gas are coupled through the boundary conditions at the liquid-gas interface with normal $\mathbf{n}$ pointing into the liquid phase. These are a kinematic equation and the standard balance of capillarity with stress acting from the two phases:

$$\mathbf{u}_l\cdot\mathbf{n} = \mathbf{u}_g\cdot\mathbf{n} = 0, \quad \mathbf{n}\cdot(\mathbf{P}_l - \mathbf{P}_g) = \sigma\mathbf{n}\nabla\cdot\mathbf{n}, \qquad (1)$$

with $\sigma$ the constant surface tension of the liquid-gas interface.

These equations are combined with a condition relating the tangential velocities on either side of the interface. This can be written in the general form

$$-A\,\alpha\,\ell\,\mu_g^{-1}\,\mathbf{n}\cdot\mathbf{P}_g\cdot(\mathbf{I}-\mathbf{nn}) = \mathbf{u}_{g,\parallel} - \mathbf{u}_{l,\parallel},$$

where the minus sign occurs because the normal points into the liquid. By setting $A = 0$, the usual condition of velocity continuity across the interface is recovered, which is used in the *no-slip model*, whereas for the *slip model* $A = 1$ is required to account for a Knudsen layer.

*Liquid-solid-gas contact line.* Equation (1) requires a boundary condition at the contact line which is given by prescribing the contact angle $\theta$. Here, the focus is on understanding the effects of the gas dynamics on the dynamic wetting flow so that the simplest option of fixing $\theta = \theta_e$ to its equilibrium value is taken. More complex implementations, such as those based on the interface formation theory [3] or the molecular kinetic theory of wetting [4], have already been built into this code [5] and so can be considered in future research.

*'Far field' conditions.* The flow configuration is sketched in Figure 1 of the Letter. At a distance $L$ from the solid surface there is a symmetry boundary at which impermeability $\mathbf{u}\cdot\mathbf{n} = 0$ and zero tangential stress $\mathbf{n}\cdot\mathbf{P}\cdot(\mathbf{I}-\mathbf{nn}) = \mathbf{0}$ must be satisfied. To ensure its smoothness, the free surface meets the plane of symmetry perpendicularly.

At the top and bottom of the domain, a distance $\pm 2L$ from the undisturbed flat free surface, are located no-slip solids. In the dip coating setup, the 'far field' boundaries are sufficiently far from the contact line to have no effect, but when the influence of meniscus confinement are considered, the presence of these boundaries, particularly the plane of symmetry, becomes important.

### Lubrication Formulation

The simulation results in the Letter have been obtained using a one-dimensional lubrication formulation in the gas phase which can be obtained in the limit $h/L \to 0$. In this approach, the pressure in the gas phase is determined by solving the lubrication equation presented in the Letter

$$-\frac{h^2}{12\,r\mu_g}\frac{\mathrm{d}p_g}{\mathrm{d}x} = \frac{U+U_{fs}}{2}, \quad r(Kn) = \frac{\sqrt{\pi}}{12Kn\,Q(Kn)}, \qquad (2)$$

where, $U_{fs} = -\mathbf{u}_l \cdot \mathbf{t}_l$ (usually $> 0$) is the liquid's velocity tangential to the free surface and $\mathbf{t}_l$ is the tangent in the direction of increasing $s$. This equation requires one boundary condition on $p$ and as the gas is assumed incompressible $p \to 0$ as $s \to \infty$ is applied (in practise, at the end of the free surface). It is further assumed that $dx \approx ds$, an approach developed in [6] and first implemented in this context in [7], where it was shown to be highly accurate for coating flows; the Benchmark Simulations also confirm this.

In the lubrication formulation [8], the pressure and tangential stress in the gas can both enter the free surface boundary conditions. However, with $\mu_g/\mu_l \ll 1$ for liquid-gas systems, it is likely that the tangential stress contribution will be negligible, and the Benchmark Simulations confirm this, so that $\mathbf{P}_g \approx -p_g\mathbf{I}$ in (1). Therefore, the coupling between the liquid and gas is through (a) the $U_{fs}$ entering (2) and (b) $p_g$ entering (1).

The assumption that $dx \approx ds$ breaks down both (a) far away from the contact line where the free surface flattens out due to gravity and (b) close to the contact line, where a region of large curvature exists in order for the free surface to meet the solid at a contact angle $\theta$ which is $\leq 90°$ in this Letter. It is not surprising that (a) is irrelevant, as in this region there is no thin film ($h \approx L$) and the gas' influence on the free surface is negligible. In contrast, it is perhaps surprising that what happens very close to the contact line does not effect the values of $U_{max}$ obtained, as confirmed in Benchmark Simulations. However, this aligns with current thinking on the mechanisms for gas entrainment [9], that it is the flow dynamics at the inflection point on the free surface that determine $U_{max}$, and this point is well outside the region of large curvature in all of the cases considered. In other words, because the inflection point is in the thin film region, the dynamics there are well captured and hence $U_{max}$ is accurately predicted.

**Method for Determining $r(Kn)$**

The function $r = r(Kn) = \frac{\sqrt{\pi}}{12Kn\,Q(Kn)}$ in (2) is obtained from $Q = Q(Kn)$, the standard 'flow coefficients' for plane pressure-driven Poiseuille flow through a channel of height $h$. Here, a variational approach developed in [10] and extended in [11] has been implemented, which uses the linearised BGK approximation to the full Boltzmann equation. In [12], the various methods of computing $Q$ are compared and the variational approach is recommended as it gives values for $Q$ that are within a couple of percent of those obtained from directly solving the Boltzmann equation [13], at a fraction of the computational cost. As a first step, it is assumed that a Maxwell condition applies at both boundaries with purely diffuse reflection, so that the accommodation coefficient on each surface is unity.

In order to pre-compute the function $r(Kn)$ for all possible values of $Kn$, asymptotic results are used which are

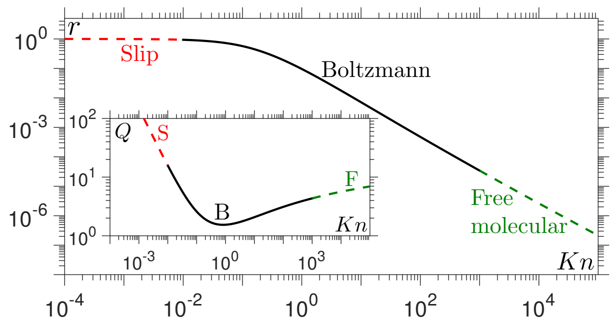


FIG. 1. Figure showing how the asymptotic expressions for $Q$ and $r$ are used when $Kn \leq 10^{-2}$ and $Kn \geq 10^3$.

accurate for $Kn \to 0$ and $Kn \to \infty$, with values computed from the variational approach patching up the gap in between where the asymptotics are inaccurate. In particular, for $Kn \leq 10^{-2}$ the slip solution [14] is used

$$r(Kn) = \frac{1}{1 + 6\alpha Kn} \qquad \text{for} \qquad Kn \leq 10^{-2},$$

with $\alpha = 1.15$ for the BGK approximation.

For $Kn \geq 10^3$ an expression derived in [15] for 'free molecular flow' is implemented, that $Q = \frac{1}{\sqrt{\pi}} \ln Kn + A$, where $A = 0.44$ is a subdominant constant term which is fitted to ensure continuity of the curve at $Kn = 10^3$, in order to give

$$r(Kn) = \frac{\pi}{12Kn(\ln Kn + 0.44\sqrt{\pi})} \qquad \text{for} \qquad Kn \geq 10^3.$$

In the range $10^{-2} < Kn < 10^3$, values for $Q$ and hence $r$ are computed, stored in a file `rvalues.txt` and quadratic interpolation is used between these points. The output of the function is shown in decomposed form in Figure 1. In this way, a function has been constructed which will work for any $Kn$ and this been implemented into the computations. Attached is a self-explanatory matlab function `r.m` which recreates $r(Kn)$ and uses the file `rvalues.txt` so that the reader can implement these kinetic effects into their own codes.

It is possible to relax the assumption of diffuse reflection on each interface but this leads to a considerably more complex formulation both for the Poiseuille flow, where the coefficients can still be obtained from the variational approach, but also for the Couette component which will no longer have the simple form presented if the two surfaces have different accommodation coefficients [16]. This could be the subject of future work.

## BENCHMARK SIMULATIONS

To establish the limits of applicability of the lubrication approach, it is compared to calculations which account for the entire two-dimensional gas flow. To align with previous work in [1], in which good agreement was

| $\mu_g/\mu_l$ | $Ca_{max}$ | | |
|---|---|---|---|
| | Full 2D | 1D in gas including tangential stress | 1D in gas excluding tangential stress |
| $10^{-1}$ | 0.09 | 0.08 | 0.07 |
| $10^{-2}$ | 0.21 | 0.21 | 0.20 |
| $10^{-3}$ | 0.39 | 0.39 | 0.39 |
| $10^{-4}$ | 0.65 | 0.65 | 0.65 |

TABLE I. Comparison of the critical capillary numbers $Ca_{max}$ obtained from the code (and hence also [18]) across a range of viscosity ratios $\bar{\mu}$ for both full 2D calculations in the gas phase as well as the lubrication formulation with and without the tangential stress incorporated into (1).

shown with simulations from [17], consider Stokes flow in both phases; with the slip-lengths of the liquid-solid and gas-solid interfaces equal at $l_s/L_\sigma = \ell/L_\sigma = 10^{-4}$ ($\alpha = 1$); no-slip across the liquid-gas interface, so that $A = 0$; a constant contact angle of $\theta = 90°$ and a domain size $L = 10L_\sigma$. Using these parameters, the maximum speed of wetting, written as a capillary number $Ca_{max} = \mu_l U_{max}/\sigma$ is computed for different viscosity ratios $\mu_g/\mu_l = 10^{-1}$, $10^{-2}$, $10^{-3}$, $10^{-4}$ using the lubrication formulation, and compared to previous results obtained with the entire gas dynamics accounted for.

In Table I, the full gas model is compared with both a lubrication approach which (a) includes the tangential stress contribution from the gas phase in (1) and (b) contains only the pressure contribution. As one can see, for $\mu_g/\mu_l \leq 10^{-2}$, which incorporates all liquid-gas systems of interest, it is reasonable (a) to assume $dx \approx ds$ and (b) take $\mathbf{P}_g \approx -p_g\mathbf{I}$ in (1). However, this formulation begins to breakdown as $\mu_g \approx \mu_l$, so that it is unlikely to be accurate for liquid-liquid systems or as an approach in both phases, as shown in [17]. Simulations were also run for the *slip model*, with $A = 1$, and similar levels of accuracy were observed.

## CONFINED MENISCI

Consider whether reducing $L$ (Figure 1 of the Letter) can introduce kinetic effects at atmospheric pressure. Stokes flow is used to isolate these effects, so that the influence of $L$ on the Reynolds number is removed, with $\mu_g/\mu_l = 10^{-4}$, air as the gas ($\ell_{atm} = 70$ nm, $\mu_g = 18\mu$Pa s), and a neutral wetting angle $\theta_e = 90°$.

Figure 2 shows that the increase in $U_{max}$ with confinement, discovered and described in detail in [17], is model-dependent. The no-slip model becomes poor for $L < L_\sigma \approx 1$mm, so that a slip model is required, whilst for $L < 0.1L_\sigma \approx 100\ \mu$m the Boltzmann model is required to fully capture the gas dynamics. In other words, full kinetic effects are required for 'microfluidic flow', which could either be a meniscus confined to a microchannel or when the bulk flow creates regions of large curvature, as in drop impact.

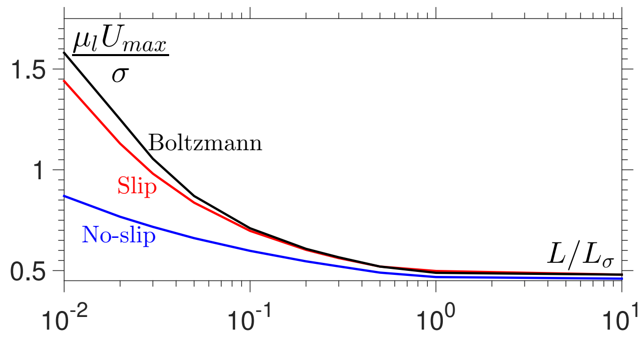


FIG. 2. Comparison of the models' predictions for the maximum speed of wetting $U_{max}$ as the domain size $L$ is decreased. Dimensionless units $Ca_{max} = \mu U_{max}/\sigma$ and $L/L_\sigma$ are used.

* J.E.Sprittles@Warwick.ac.uk

[1] J. E. Sprittles, J. Fluid Mech. **769**, 444 (2015).
[2] Within the range of experimentally measured values [**?** ].
[3] Y. D. Shikhmurzaev, *Capillary Flows with Forming Interfaces* (Chapman & Hall/CRC, Boca Raton, 2007).
[4] T. D. Blake and J. M. Haynes, J. Coll. Int. Sci. **30**, 421 (1969).
[5] J. E. Sprittles and Y. D. Shikhmurzaev, J. Comp. Phys. **233**, 34 (2013).
[6] D. Jacqmin, J. Fluid Mech. **517**, 209 (2004).
[7] E. Vandre, Ph.D. thesis, University of Minnesota (2013).
[8] A. Oron, S. H. Davis, and S. G. Bankoff, Rev. Mod. Phys. **69**, 931 (1997).
[9] E. Vandre, M. S. Carvalho, and S. Kumar, J. Fluid Mech. **747**, 119 (2014).
[10] C. Cercignani and C. D. Pagani, Phys. Fluids **9**, 1167 (1966).
[11] C. Cercignani, M. Lampis, and S. Lorenzani, Phys. Fluids **16**, 3426 (2004).
[12] F. Sharipov and V. Seleznev, J. Phys. Chem. Ref. Data **27**, 657 (1998).
[13] K. A. Hickey and S. K. Loyalka, J. Vac. Tech. A **8**, 957 (1990).
[14] N. G. Hadjiconstantinou, Phys. Fluids **18**, 111301 (2006).
[15] C. Cercignani and A. Danieri, J. Appl. Phys. **34**, 3509 (1963).
[16] C. Cercignani, "Slow rarefied flows: Theory and application to MEMS," (Birkhauser, 2006).
[17] E. Vandre, M. S. Carvalho, and S. Kumar, J. Fluid Mech. **707**, 496 (2012).
[18] E. Vandre, M. S. Carvalho, and S. Kumar, Phys. Fluids **25**, 102103 (2013).
